# Supplementary material for: From structure mining to unsupervised exploration of atomic octahedral networks
Source: arXiv:2306.12272 ancillary file (2026-03-17)
Supplement: Supplementary file 1 [file Crystmorph_SI_Table5.pdf]

**Supplementary Table 5** Illustrations of common inorganic framework polytypes from the hybrid iodoplumbate dataset. Only one material is provided for each polytype with its index (CSD\_ID) from the Cambridge structure database (CSD).

| Index | Polytype name         | CSD_ID  | Chemical formula                                                                      | Variability                                                                                               | Structure example                                                                     |
|-------|-----------------------|---------|---------------------------------------------------------------------------------------|-----------------------------------------------------------------------------------------------------------|---------------------------------------------------------------------------------------|
| 1     | 2D CS layer           | 2051120 | C <sub>4</sub> H <sub>16</sub> I <sub>4</sub><br>N <sub>2</sub> Pb S <sub>2</sub>     | Number of stacked perovskite layers can vary (1-6); relative spatial translation can occur between layers | 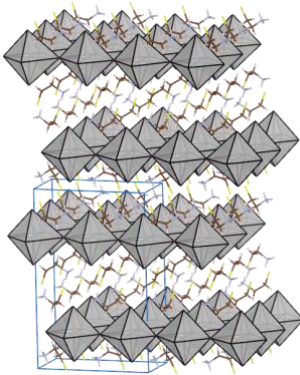   |
| 2     | FS chain              | 1844581 | C <sub>16</sub> H <sub>35</sub><br>I <sub>6</sub> N <sub>3</sub> O<br>Pb <sub>2</sub> | Number of FS chains per unit cell can vary                                                                | 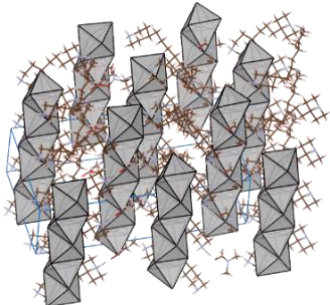  |
| 3     | 3D CS perovskite      | 1993905 | C H <sub>5</sub> I <sub>3</sub><br>N <sub>2</sub> Pb                                  |                                                                                                           | 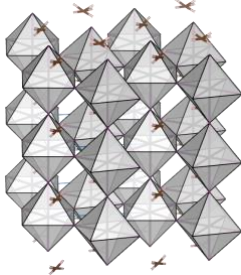 |
| 4     | ES chain of ES 2-mers | 1427135 | C H <sub>8</sub> I <sub>3</sub> N<br>O Pb                                             | Neighboring ES 2-mers may be connected by different edges                                                 | 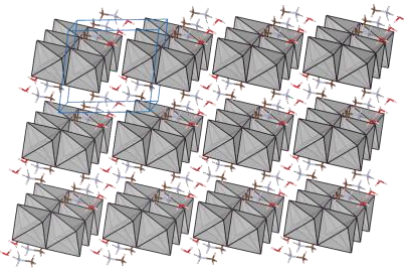 |
| 5     | isolated (1-mer)      | 2034767 | C <sub>4</sub> H <sub>24</sub> I <sub>6</sub><br>N <sub>12</sub> Pb                   | Number of octahedra per unit cell may vary                                                                | 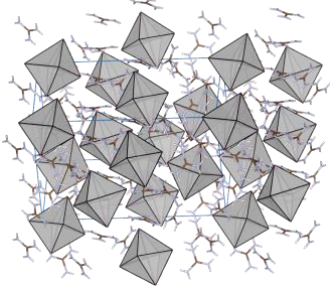 |

|    |                                             |             |                                           |                                |                                                                                       |
|----|---------------------------------------------|-------------|-------------------------------------------|--------------------------------|---------------------------------------------------------------------------------------|
| 6  | ES chain<br>of FS 3-<br>mers                | 9573<br>18  | C20 H44<br>I10 N4<br>Pb3                  |                                | 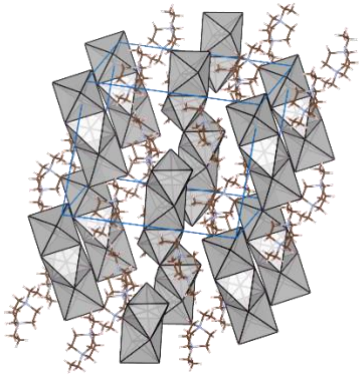   |
| 7  | 2D CS<br>corrugate<br>d layer               | 1548<br>809 | C2 I4 N6<br>Pb                            | CS layer thickness<br>may vary | 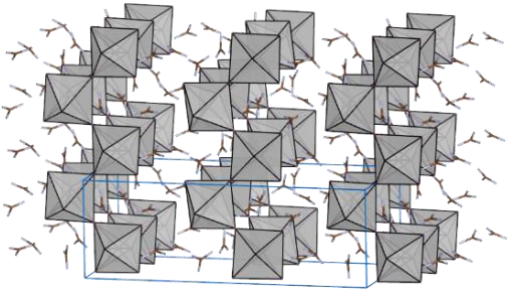   |
| 8  | CS chain<br>of ES 2-<br>mer of FS<br>2-mers | 1537<br>07  | (C12 H26<br>N2<br>2+)2n,n(I1<br>2 Pb4 4-) |                                | 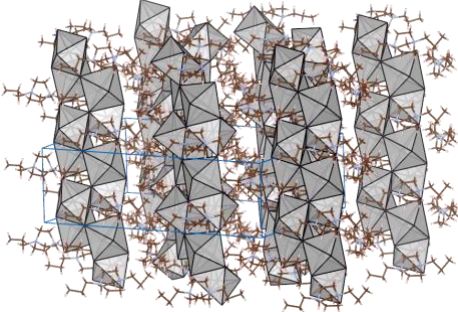  |
| 9  | CS zigzag<br>chain                          | 1910<br>573 | 2(I10<br>Pb2),<br>12(C3 N)                |                                | 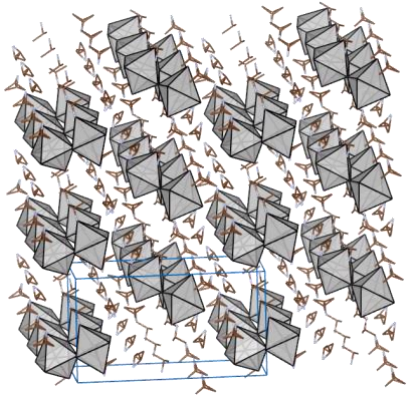 |
| 10 | CS layer<br>of FS 3-<br>mers                | 2053<br>587 | 4(C7 H14<br>N O2), I10<br>Pb3             |                                | 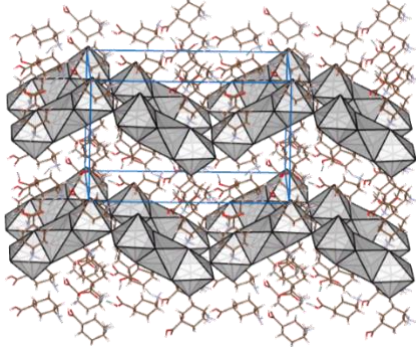 |

|    |                              |             |                                      |                                                                                                           |                                                                                       |
|----|------------------------------|-------------|--------------------------------------|-----------------------------------------------------------------------------------------------------------|---------------------------------------------------------------------------------------|
| 11 | CS chain                     | 1505<br>390 | I5 Pb, C2<br>H6 O S,<br>3(C H6 N)    |                                                                                                           | 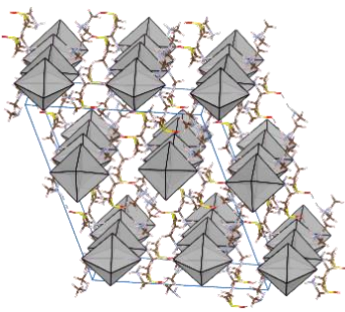   |
| 12 | FS 3-mer                     | 1519<br>639 | C36 H46<br>I12 N12<br>O2 Pb3         |                                                                                                           | 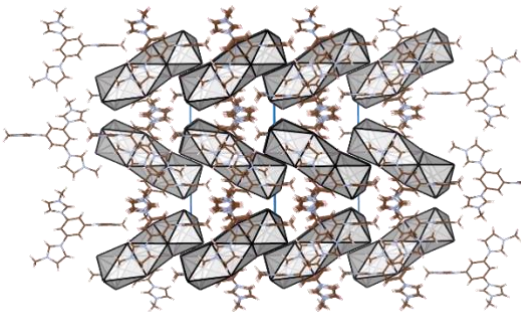    |
| 13 | ES chain<br>of ES 3-<br>mers | 7659<br>30  | C24 H33<br>I9 N3 Pb3                 | Location of<br>connections<br>between ES 3-<br>mers may vary                                              | 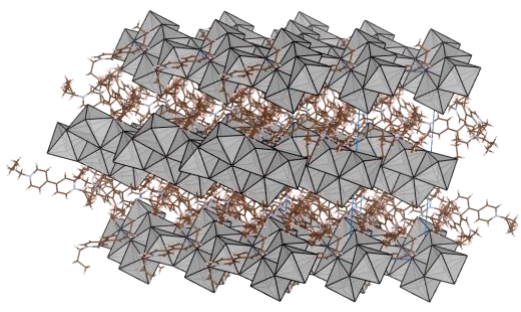   |
| 14 | CS chain<br>of CS 3-<br>mers | 2116<br>341 | C96 H115<br>I14 N8 O2<br>Pb3         | Multiplicity of<br>secondary building<br>unit can vary from<br>2 to 5 (3-mer<br>being the most<br>common) | 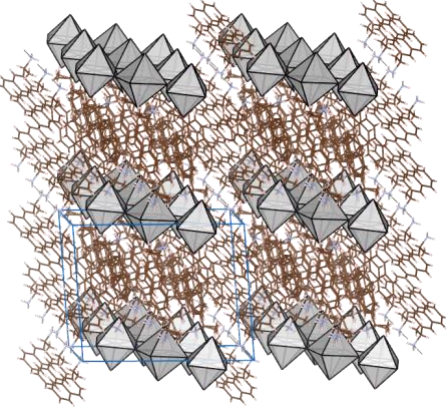 |
| 15 | ES chain                     | 6329<br>22  | (C6 H10<br>N2) [Pb<br>I4] , 2H2<br>O | Number of ES<br>chains per unit cell<br>can vary                                                          | 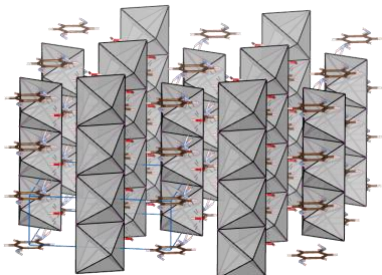 |

|    |                                       |          |                        |                                                  |                                                                                       |
|----|---------------------------------------|----------|------------------------|--------------------------------------------------|---------------------------------------------------------------------------------------|
| 16 | CS framework of CS layer of ES 2-mers | 2074 690 | 0.5(I12 Pb4), C6 H8 N4 | The tilting angle between ES 2-mers may not be 0 | 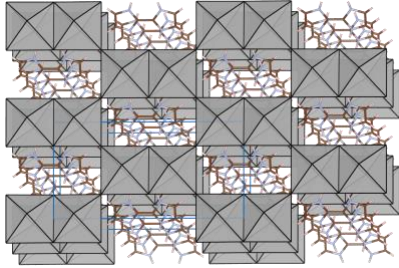   |
| 17 | CS layer of FS 2-mers                 | 1937 882 | C9 H30 I7 N3 Pb2       |                                                  | 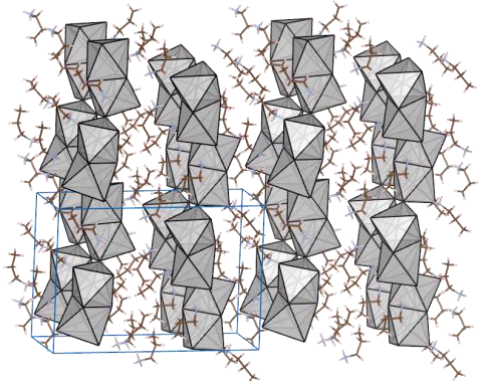   |
| 18 | CS corrugated layer of ES 2-mers      | 1880 804 | C H5 I5 N2 Pb2 S       |                                                  | 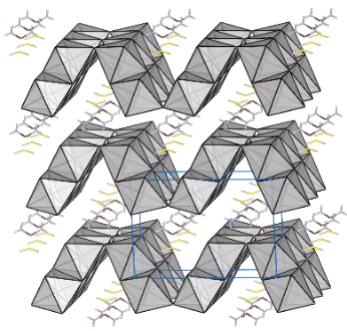  |
| 19 | ES 5-mer chain                        | 1549 803 | C28 H44 I14 N4 O2 Pb5  |                                                  | 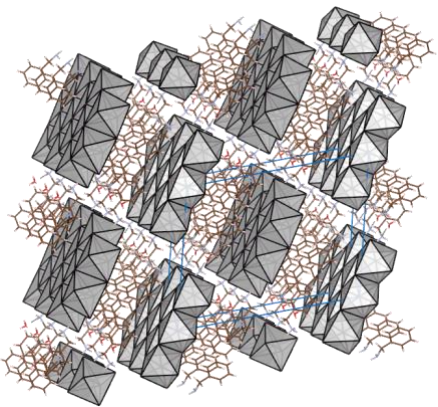 |

|    |                                          |             |                                            |                               |                                                                                       |
|----|------------------------------------------|-------------|--------------------------------------------|-------------------------------|---------------------------------------------------------------------------------------|
| 20 | ES layer                                 | 2080<br>61  | C8 H4 I5<br>Pb1.25<br>S6                   | ES layer may be<br>corrugated | 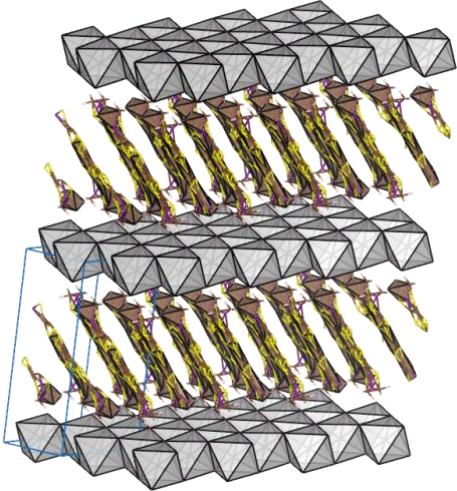   |
| 21 | FS chain<br>of FS<br>curved 6-<br>mers   | 7071<br>69  | C18 H42<br>N6 O8 Y,<br>I9 Pb3              |                               | 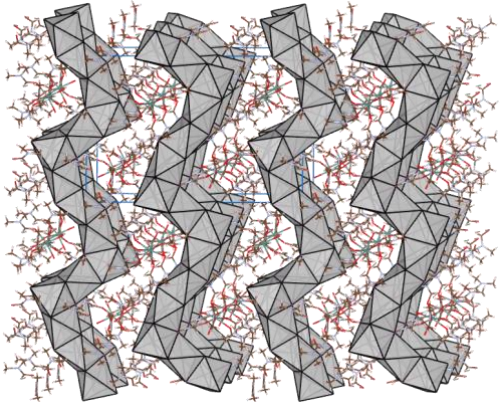  |
| 22 | CS layer<br>of FS<br>circular 3-<br>mers | 1902<br>194 | C8 H19 I9<br>N2 Pb3                        |                               | 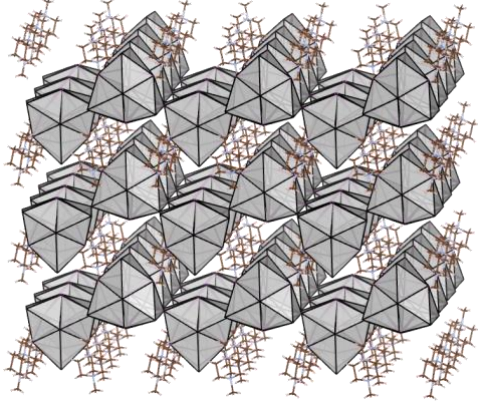 |
| 23 | CS layer<br>of CS-ES<br>3-mers           | 1838<br>614 | I21 Pb5,<br>6(C6 H10<br>N2), I,<br>3(H2 O) |                               | 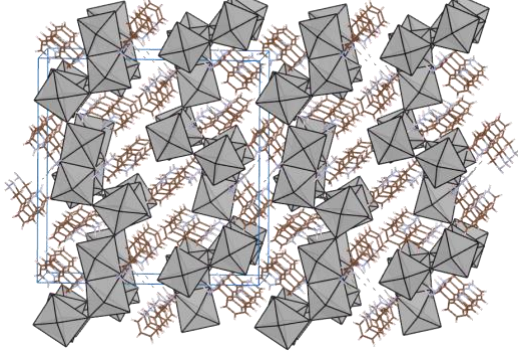  |

|    |                              |             |                                     |  |                                                                                       |
|----|------------------------------|-------------|-------------------------------------|--|---------------------------------------------------------------------------------------|
| 24 | FS 2-mer                     | 1997<br>919 | C7 H42 I9<br>N7 Pb2                 |  | 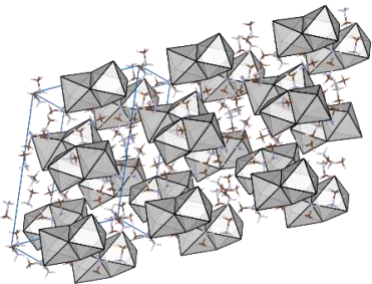   |
| 25 | CS chain<br>of ES 2-<br>mers | 2125<br>046 | C12 H32<br>I8 N4 O2<br>Pb2          |  | 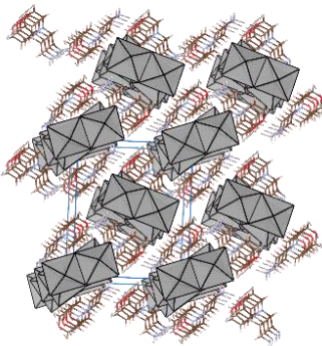   |
| 26 | FS chain<br>of FS 3-<br>mers | 1063<br>784 | C27 H32<br>I9 N3 O<br>Pb3           |  | 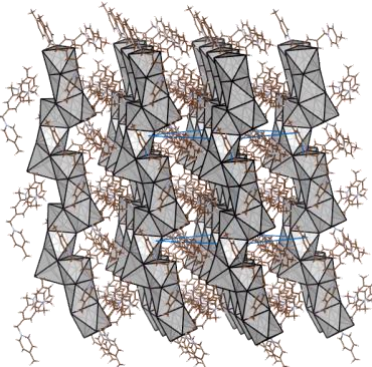  |
| 27 | CS chain<br>of CS 2-<br>mers | 1880<br>798 | C5 H27 I9<br>N8 Pb2<br>S3           |  | 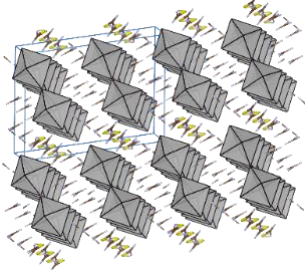 |
| 28 | CS chain<br>of CS 5-<br>mers | 6252<br>35  | C24 H92<br>I22 N12<br>O4 Pb5<br>S12 |  | 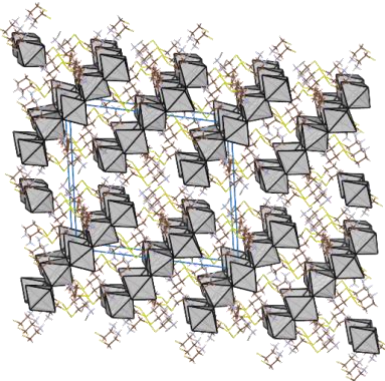 |
